# Supplementary material for: Exploration in Feature Space for Reinforcement Learning
Source: arXiv:1710.02210 source file (2017-10-05)
Supplement: Supplementary file 1 [file appendix.tex]

% \appendix
